# Supplementary material for: Effects of Spin-Orbit Coupling and Thermal Expansion on the Phonon-limited Resistivity of Pb from First Principles
Source: arXiv:2410.20157 source file (2025-03-11)
Supplement: Supplementary file 1 [file appendix.tex]

\appendix
\counterwithin{figure}{section}

% \section{Extra Pb data}

% This is extra data for Pb.
% \begin{figure}
%     \centering
%     \includegraphics[width=\columnwidth]{figures/Pb/extra/ph_disp_kgrid_conv_vs_exp_noSOC.pdf}
%     \caption{Phonon dispersion convergence without SOC compared to experimental data.}
%     \label{fig:Pb_phonon_dispersion_kgrid_convergence_noSOC}
% \end{figure}

% \begin{figure}
%     \centering
%     \includegraphics[width=\columnwidth]{figures/Pb/extra/ph_disp_kgrid_conv_vs_exp.pdf}
%     \caption{Phonon dispersion convergence with SOC compared to experimental data.}
%     \label{fig:Pb_phonon_dispersion_kgrid_convergence_SOC}
% \end{figure}
